# Supplementary material for: Sequential Neural Barriers for Scalable Dynamic Obstacle Avoidance
Source: arXiv:2307.03015 source file (2023-07-06)
Supplement: Supplementary file 1 [file appendix.tex]

\section{Algorithm}

\begin{algorithm}[h!]
\caption{Boundary refinement for neural CBF models}
\label{alg::training}
\begin{algorithmic}[1]
\NoThen
\State \textbf{Input}: neural CBF model $B$, neural dynamics model $\pi$, 
%nominal controller $\phi$, 
%relative obstacle state-sequence $h_{0}$, relative obstacle state-sequence at the next time step $h'$, 
threshold $\theta$, initial safe set $D_{s}$ and unsafe set $D_{u}$
% \shnote{should $\alpha$ be $\theta$ as in the text? what's the difference between $h$ and $h_0$? both used. Should $X_0$ be $D^\theta$? What is $N_s, N_u$?}
\State \textbf{Output}: updated safe set $D_{s}$ and unsafe set $D_{u}$
%\State $D_{s}, D_{u} \gets [], []$
\State $D^{\theta} \gets$ SampleBoundaryStates($D_s$, $\theta$) 
\label{algLine::alg1::sample_boundary}
\For{$(x,h)$ in $D^{\theta}$} 
\State $u \gets$ GetNominalControl($\phi$, $x$, $h$) 
\label{algLine::alg1::get_nominal_controls}
\State $x^{'} \gets \pi(x, u)$
\label{algLine::alg1::unroll_agent_nominal}
\If{($x$, $h$) or ($x'$, $h'$) violates safety constraint}
\State append $(x, h)$ and $(x', h')$ to $D_{u}$ 
% \State remove $(x,h)$ from $D_s$
% \State \textbf{continue}
% \EndIf
% \ElsIf {($x^{n}_{1}$, $h_{1}$) or ($x^{n}_{2}$, $h_{2}$) violates safety constraint}
% \State append $(x, h)$ to $X_{u}$
% \State append $(x^{n}_{1}, h^{n}_{1})$ to $X_{u}$
% \State \textbf{continue}
% \EndIf
\Else{}
\State append $(x, h)$ to $D_{s}$
\State $u \gets$ GetRandomControl($x$, $h$) 
\label{algLine::alg1::get_barrier_controls}
\State $x' \gets \pi(x,u)$ 
\label{algLine::alg1::unroll_agent_nominal}
\newdimen\origiwspc%
\origiwspc=\fontdimen2{
{($x'$, $h'$) violates safety constraint}\label{algLine::alg1::check_barrier_invariance}}%CheckSafetyViolation CheckSafetyViolation CheckAvailableBarrierControl
% \fontdimen2\font=\origiwspc
\State append ($x'$, $h'$) to $D_{u}$
\EndIf
\EndIf
\EndFor
\end{algorithmic}
\end{algorithm}

\begin{algorithm}[h!]
\caption{Online Inference}
\label{alg::planning}
\label{alg::planning}
\begin{algorithmic}[1]
\State \textbf{Input}: CBF model $B$, learned ego-dynamics model $\pi$, obstacle state sequences $h_{1}$, ..., $h_{q}$, agent state $x$, clip threshold $b$, goal-progress metric $d(\cdot)$ %, unsafe threshold $\alpha$
\State \textbf{Output}: control $u$ 
\State $u_{1}, ..., u_{l} \gets$ SampleControls()
\label{algLine::sample_candidates}
\For{$i$ in $1, ..., l$}
\State $x'_{i} \gets $ UnrollAgentDynamics($u_{i}$, $x$, $\pi$)
\label{algLine::unroll_dynamics}
\State $\hat B({x'_{i})} \gets \prod_{j=1}^q \max\bigg(\frac{1}{b}\min\Big(B(x'_{i},h_j),b\Big),0\bigg)$ 
\State $s_{i} \gets d(x'_{i}, h_{1}, ..., h_{k})$
\label{algLine::compute_scores}
\EndFor
\For{$x'_{i}$ in descending order of $s$}
\label{algLine::find_safe_begin}
% \If{$barrier\_scores[i] > \alpha$}
% % \State \textbf{return} $ACs[i]$
% \State $ac\_idx \gets i$
% \State $break$
\If{$\hat B({x'_{i}}) > 0$}
\State \textbf{return} $u_{i}$
\EndIf
\EndFor
\label{algLine::find_safe_end}
% \If{$barrier\_scores[ac\_idx]$ $==$ None}
% \label{algLine::if_too_unsafe}
% \State \textbf{return} $ACs[\arg\max(barrier\_scores)]$
% \label{algLine::return_safest}
% \Else 
% \State \textbf{return} $ACs[ac\_idx]$
% \label{algLine::return_CBF_ac}
% \EndIf
\end{algorithmic}
\end{algorithm}

\section{Experiments}

\noindent{\bf Environments.} In the robot navigation environment, an agent vehicle aims to reach a goal location without colliding with any of the pedestrians. Each pedestrian starts at random positions, and moves towards different random goals. Their interaction dynamics follows the ORCA model~\cite{ORCA}. In this model the pedestrians interact and affect each other's movement, but they do not try to avoid the ego-robot. This choice gives a focused evaluation of the control performance on the ego-robot, since it is fully responsible for safety, as the pedestrians are neither cooperative nor adversarial. Note that neither our method or the baseline methods have access to the dynamics model of the pedestrians, so other models can be easily used in the simulation engine. 
%We plan the obstacle trajectories with the ORCA model so that obstacles approach their individual goals without crashing into each other. 
%One obstacle's goal is re-selected if it is reached. 
%The agent cannot be perceived by obstacles, and is not taken into account by the ORCA. 
For the ego-robot, we experiment with different underlying dynamics to test the control performance under varying control authority, including the single-integrator, double-integrator, Dubins car, and the bicycle model. We do not access the analytic form of the robot dynamics, and will show how the different underlying dynamics significantly affects the neural CBFs through model-free learning. We perform training with a small number of pedestrians and evaluate the performance in environments with up to 100x the density. 

The lane-changing environment contains a multi-lane highway. The ego-vehicle needs to maintain speed and perform lane changing when needed, while avoiding crashing other vehicles. The surrounding vehicles start from random positions and then follow the intelligent driver model (IDM)~\cite{treiber2000congested}. The underlying dynamics of the ego-vehicle uses the kinematic bicycle model. The lane structure of this environment allows us to better compare with deep Q-learning methods, which are hard to scale in the robot navigation environment.

\noindent{\bf Potential Field Design.} To evaluate the proposed method, we employ a potential-field controller to acquire reference controls. We also assess its performance as one of the baselines. Denote the goal and obstacle state with $s_{goal}$ and $s_{obs}$ respectively. With the Euclidean distance metric $d$,  we compute the potential field at one arbitrary agent state $s$, by composing the repulsive and the attractive fields as follows:
\begin{equation}
\label{eqn::potential_field}
\begin{split}
% \begin{align*}
    U(s) &= U_{att} (s) + \sum_{s_{obs}}U_{rep} (s, s_{obs}),  \\ 
    U_{att}(s) &= \frac{1}{2} \zeta d(s, s_{goal}), \\ 
    U_{rep}(s, s_{obs}) &= \begin{cases}
      \frac{1}{2} \eta (\frac{1}{d(s, s_{obs})} - \frac{1}{Q^{*}})^{2} & \text{, $d(s, s_{obs}) \leq Q^{*}$,} \\ 
      0 & \text{, $d(s, s_{obs}) > Q^{*}$,}
    \end{cases}       
\end{split}
\end{equation}
% \end{align*}
where $\zeta$ and $\eta$ are the weighting coefficients, and $Q^{*}$ represents the distance of influence for the repulsive field. To adapt to the settings with moving obstacles, we predict the future obstacle states with a neural network trained separately from offline procedures. Then the potential fields are computed based on the obstacle positions predicted at the next time-step.

\indent{\bf Training Setup and Parameters.} We only perform learning in environments with a small number of dynamic obstacles: in the navigation environment we train with only 6 pedestrians, and in the lane-changing environment with 6 vehicles. 

To train the neural CBFs, we choose $\gamma = 10^{-2}$ as the learning error margin parameter in \ref{eqn::barrier_objective}, and select the extended class-$\mathcal{K}_{\infty}$ function for the CBF to be $\alpha(x) = 0.1 x$. In the first training phase, we approximate the barrier function by optimizing (\ref{eqn::barrier_objective}) with offline inference procedures collected with the sampling-based potential-field controller as the nominal controller. 
We collect $1000$ collision-free trajectories as demonstrations, which contains $50,000$ state-action pairs. 
In the second phase of refinement training, we include $1,000$ random state-action pairs from the first phase in each episode. For every obstacle state-sequence in the random pairs,  we sample $100$ states around the safety boundary determined by the first phase, with a boundary threshold of $\theta = 0.05$. 
%\todo{is 100 the total boundary samples? or just one episode? how many in total?} 
% To prevent overfitting, we also include $1,000$ random state-action pairs from the first phase, and use a boundary threshold of $\theta = 0.05$. 
After obtaining the new safe and unsafe set as described in Section \ref{section::learning}, we train the neural CBF for $2,000$ iterations. 
%The neural network sizes... \todo{fill in}
The LSTM model we use has $64$ hidden units, the MLP model that encodes agent states has $2$ layers by $64$ neurons, and the final MLP has $2$ layers by $128$ neurons. 
We terminate the refining when the objective reaches convergence across epochs. The training typically progresses quickly, with typical learning curves as illustrated in Fig.~\ref{fig::nav_training_logs}. In performing online inference with the neural CBF, we clip barrier values to be below $b = 0.5$. %\todo{mention the b parameter here}

Figure \ref{fig::nav_training_logs} shows an example of the learning curves in the training of the neural CBF model in the navigation envionment, where the ego-robot uses the Dubins vehicle dynamics. The learning procedures typically converge quickly as shown across all environment settings. Figure \ref{fig::refinement_example} shows one concrete example of how the refinement procedures improve the landscape learning.

%the Dubins vehicle dynamics in navigation environment. The learning steps typically converge quickly. 
%\shnote{what do you mean by ``in navigation?''} 

%It suggests that the neural barrier is generalizable enough to handle the unseen new samples in the barrier boundary. 
%More importantly, the neural barrier satisfies the CBF conditions, given the low loss the model converges to.

\begin{figure}[ht]
\centering
\includegraphics[width=0.32\textwidth]{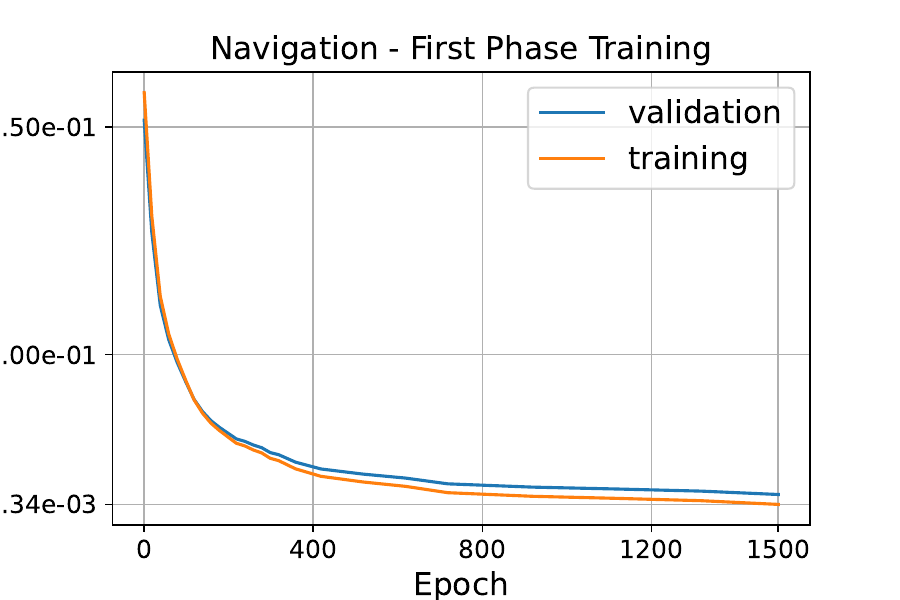}
\includegraphics[width=0.32\textwidth]{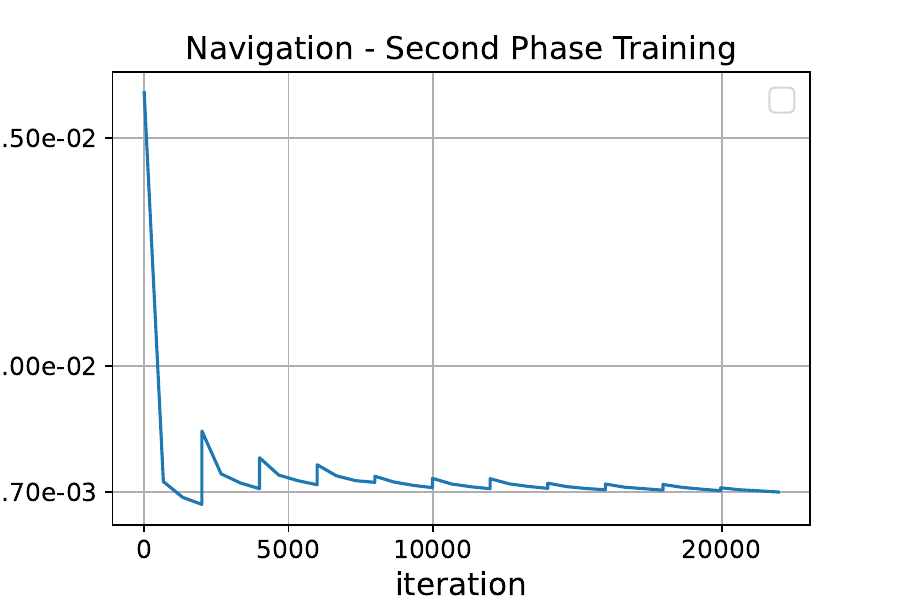}
\includegraphics[width=0.32\textwidth]{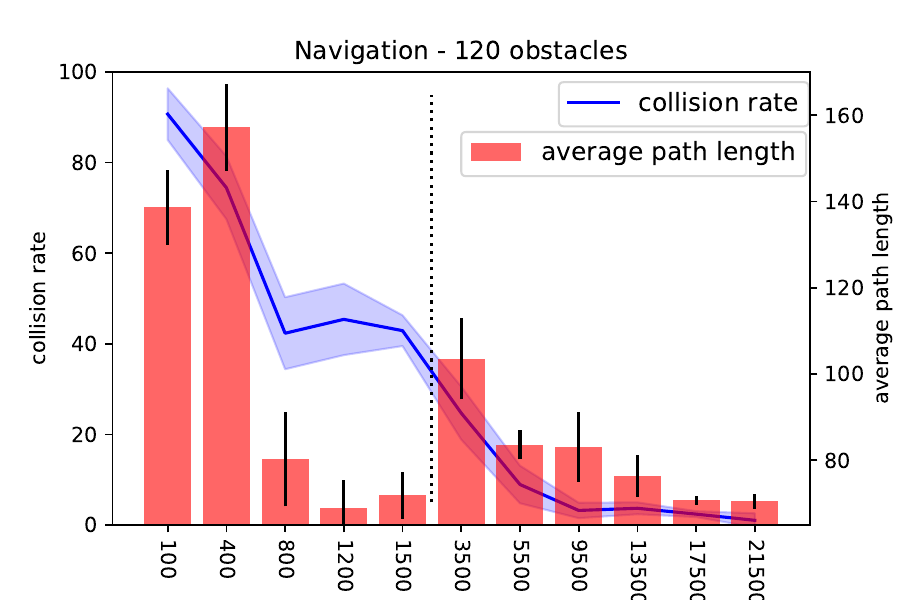}
\caption{{(\bf Plot 1-2)}The learning curves for two phases in the navigation environment with 6 dynamic obstacles and the ego-robot follows Dubins car dynamics. Note that the initial loss at the second phase is relatively high and can be quickly reduced further, after updating the dataset. {\bf (Plot 3)} Test performance improves as training progresses. The vertical dashed line marks the start of boundary refinement procedures.} %\shnote{explain this is for the dubins car. Text too small}{\bf these loss are quite small in the beginning?}
\label{fig::nav_training_logs}
\end{figure}

\begin{figure}[ht]
\centering
\includegraphics[width=0.32\textwidth]{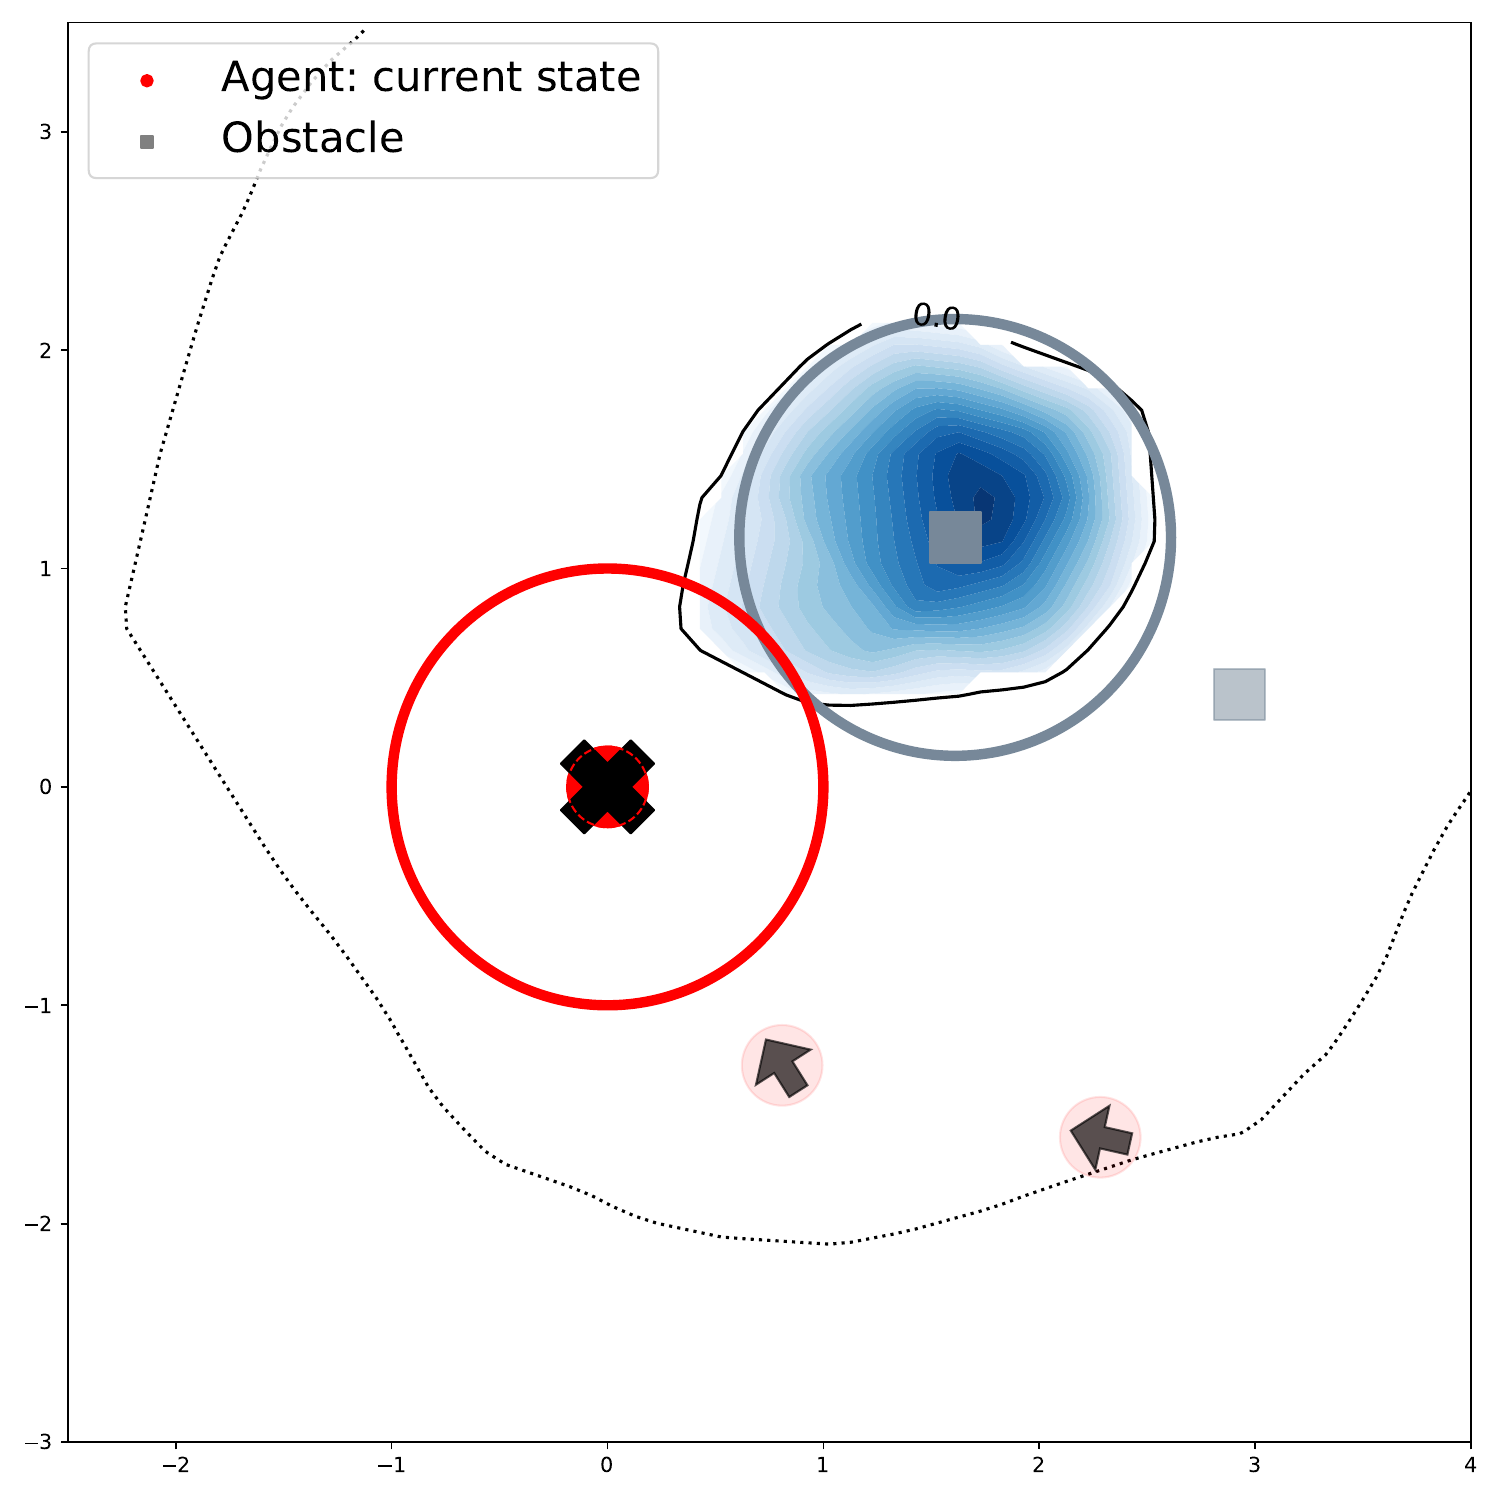}
\includegraphics[width=0.32\textwidth]{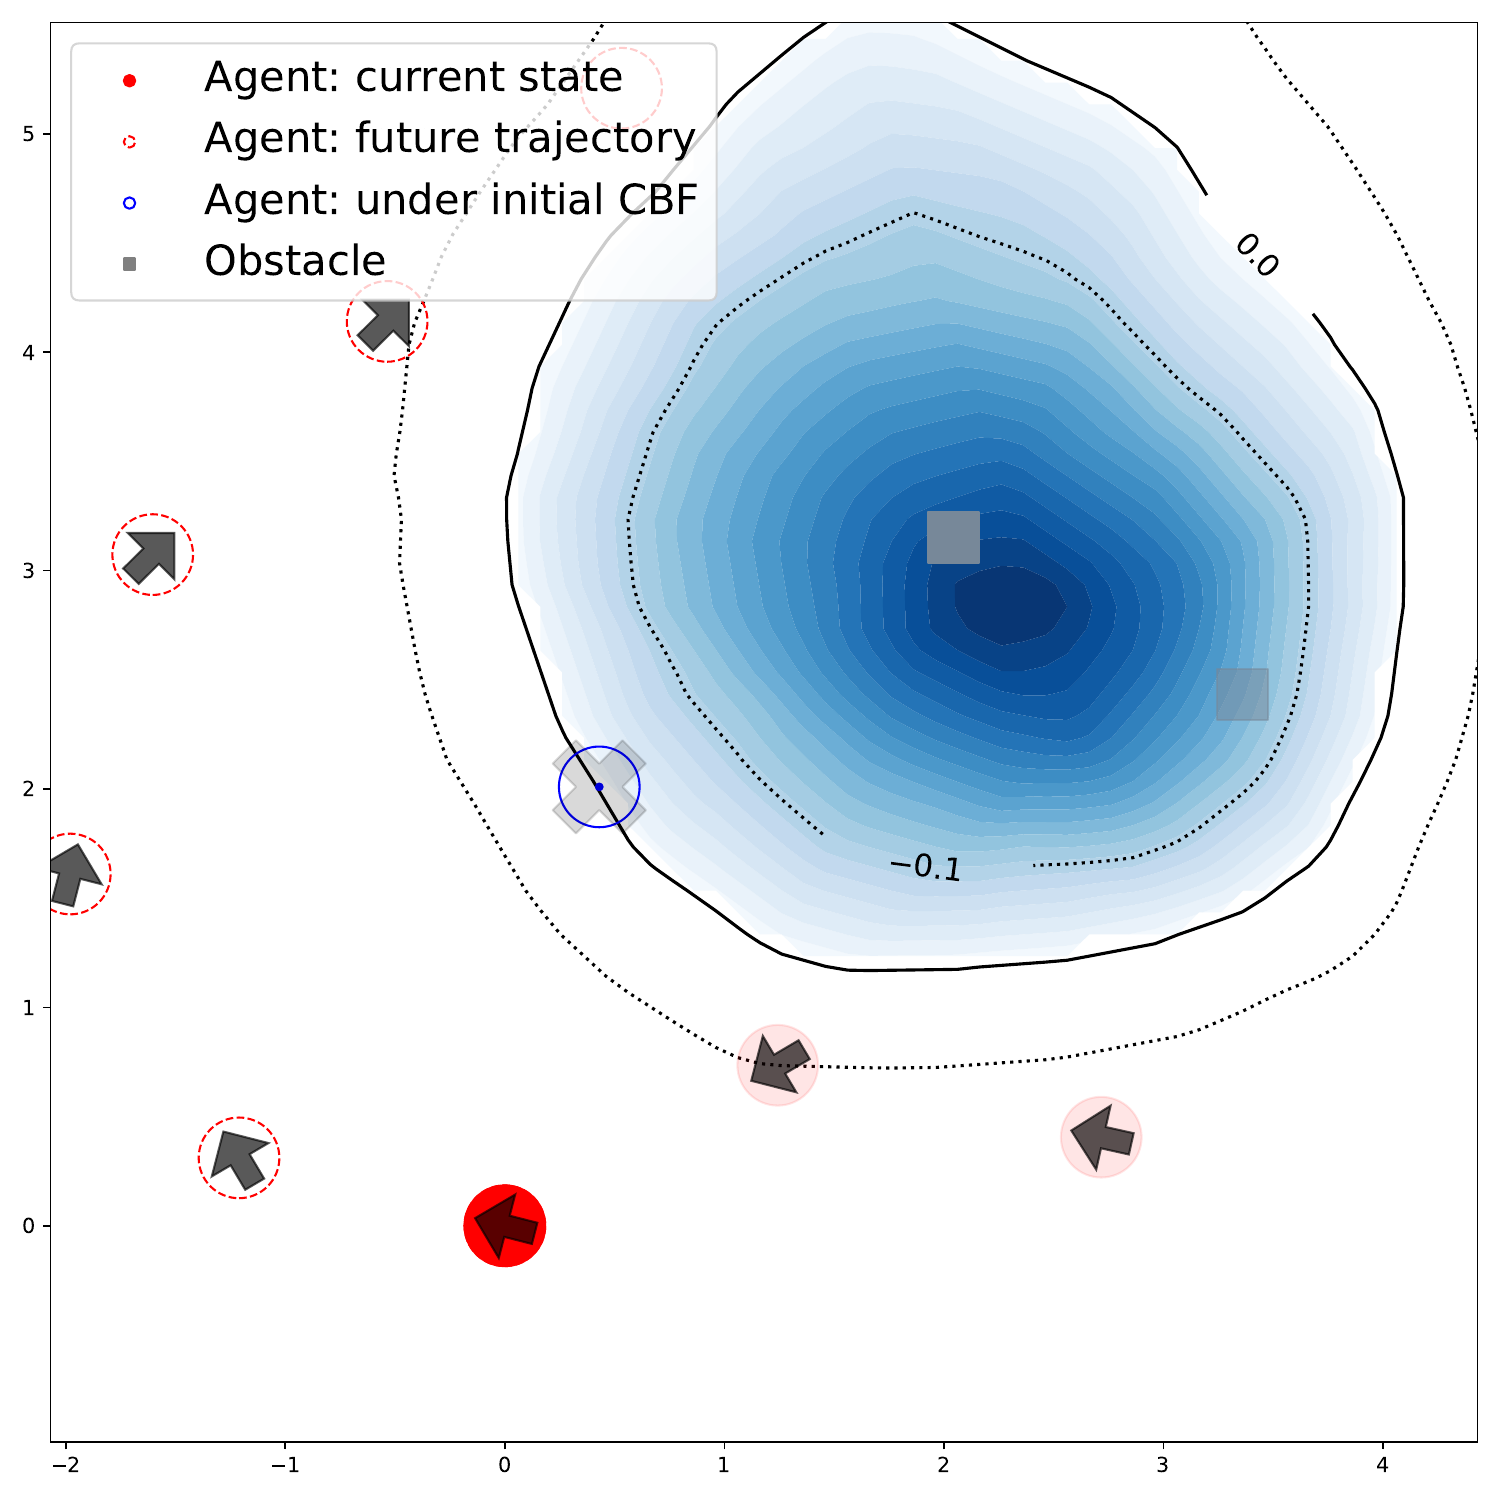}
\caption{{\bf Left:} The level sets learned from the initial training can not avoid collision at the crossed red circle. {\bf Right}: After refinement, the level sets assign more accurate values around the safety boundary, and the ego-robot (the red circles with arrows indicating directions) can avoid the obstacle using this CBF.}
\label{fig::refinement_example}
\end{figure}

\noindent{\bf Comparison with Model-Predictive Approaches.}\label{compare_mpc} The standard setting of model-predictive control (MPC) requires the use of analytic dynamics models of both the ego-robot and the obstacles to perform online optimization for control, and thus can not be directly applied to our model-free setting. However, we can still compare with a sampling-based adaptation of the model-predictive approach by sampling control actions and forward predicting the future states for multiple steps using our learned dynamics model $m$, then selecting control actions based on the potential field values of predicted states. This comparison allows us to understand the effectiveness of the CBF models in capturing the underlying dynamics without multi-step unrolling. In Figure~\ref{fig:mpc}, we show a comparison with multiple configurations of the sampling-based MPC approach. %The detailed analysis is provided in the Appendix. 

A major bottleneck for the sampling-based model-predictive approach is that the number of control actions increases exponentially in the number of unrolling steps, so we need to balance the length of the unrolling horizon and the number of sampled actions in each step. For this purpose at each predictive step in MPC, the control actions are no longer randomly sampled in the entire control action space, but are sampled around nominal controls with a Gaussian distribution. We unroll the learned dynamics model for 3 forward steps in these MPC approaches.  
%In our use of MPC controllers, the prediction horizon is $3$ future time-steps \shnote{3 what? seconds? time steps?}. 
At each step, we sample $10$ control actions based on a sampling-based potential-field controller, whose sample size is experimented with $10$ and $100$, indicated by S-MPC (10) and S-MPC (100) in Figure~\ref{fig:mpc}. We observe that the accumulation of prediction error becomes a main factor in higher collision rate as we scale up the density of obstacles. Note that S-MPC (10) requires 100 times more samples of control actions compared to neural CBF methods, and S-MPC (100) requires 1000 times more. 

%\todo{now explain the setting of each curve in the plot} 
We also compare with the best possible version of MPC that has access to the ground truth dynamics, in which we directly use the environment simulator to unroll the system instead of any learned model. This is the only case when S-MPC achieves lower collision rate than the neural CBF, and from this comparison we also see the neural CBF is able to perform close to this optimal setting of the MPC baseline (6\% vs. 9\% collision rate in the 600-obstacle environment). 

Throughout the experiments, we observe the benefits of CBF models in capturing the dynamic nature of the interaction through the barrier landscapes, so that we can avoid expensive online computation caused by the need to sample combinatorially-many control actions due to unrolling. It also allows us to avoid the accumulation of model-prediction errors that are inherent in learning-based models of dynamics. 

\begin{figure}[h]
\centering
\includegraphics[width=0.8\textwidth]{plots/fig8_combine.pdf}
\caption{(Left) Comparisons with various settings of the sampling-based Model Predictive Control (S-MPC) in the navigation environment with with Dubins car model for the ego-vehicle. (Right) Comparisons between a single CBF and the model ensemble methods in the navigation environment.}
\label{fig:mpc2}
\end{figure}

\subsection{Measuring Uncertainty with Model Ensembles}\label{section::exp_ensemble}

We now discuss how the use of model ensembles affects the control performance. 
%improves the reliability of neural barriers. Despite the ability of neural network that it can approximate any distributions by the universal approximation theorem \cite{hornik1989multilayer}, it is challenging to guarantee and verify model's generalizability to the unseen data. 
Figure \ref{fig::nav_ensemble} shows a scenario where using model ensembles can avoid unreliable value predictions from the neural CBF model. In Figure \ref{fig::nav_ensemble}, the collision at the blue circle happens, because the predicted future state of the chosen action is wrongly determined to be safe by the CBF model. We can avoid this by evaluating the uncertainty of the CBF predictions, using model ensembles. At the state that was wrongly classified by a single CBF model, we obtain the large variance on the predictions of multiple CBF models. In the plot, the curves of different colors correspond to the different level sets from multiple models. In online control, we filter out control actions that lead to states with high uncertainty, and choose other safe control actions that are able to avoid the collision. 

We also observe a trade-off between safety and false positives from model ensembles. In Figure~\ref{fig:mpc2} (Right), we see that the overall collision rate is much reduced when we use model ensembles, but much more cases of trajectory termination happen because feasible controls may be filtered out, because of the uncertainty quantification. %\shnote{verify that this is clearly seen in figure 9 because it is to small for me to tell} 
In practice, model ensembles are particularly useful for online monitoring of cases that may require human intervention.

%we plan one Dubins vehicle with a single neural barrier colored in grey. The cause of collision is that this single barrier model misclassifies this collision state as a safe one. As demonstrated by Figure \ref{fig::nav_ensemble}, the agent state falls outside this single CBF's unsafe boundary. With model ensemble, we only yield controls that most model agree on the control safety. In Figure \ref{fig::nav_ensemble}, the agent planned with barrier ensemble avoids the collision and select the control that is classified as safe by all the neural barriers. [However, the use of barrier ensemble could undermine the forward-invariance property imposed in training objective. As we train each of the component models separately, we cannot guarantee ... For instance if we exploit the barrier ensemble in an extremely conservative way, there could exist no control to reach the safe states agreed by all models.] 

\begin{figure}[h]
\centering
\includegraphics[width=0.5\textwidth]{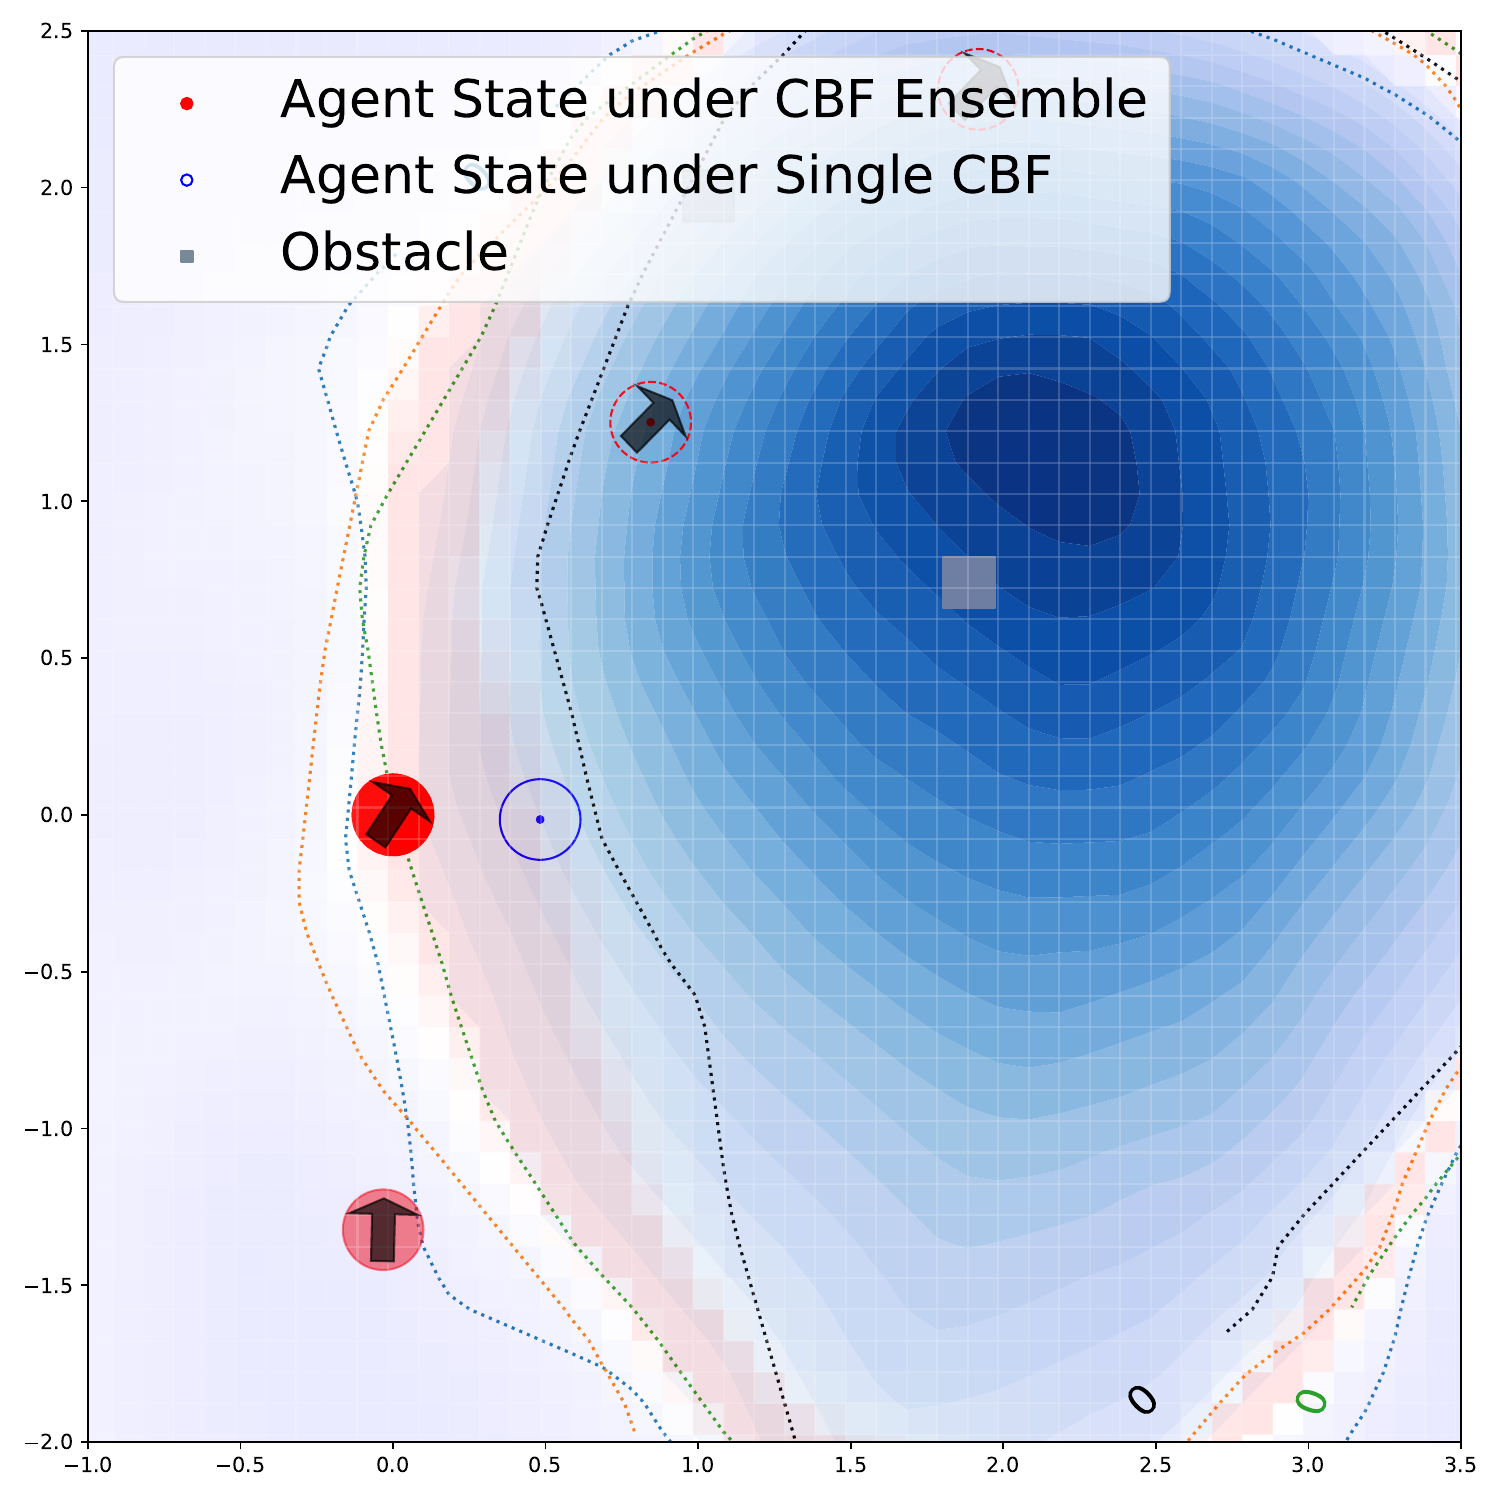}
\caption{Collision occurs with a single CBF due to the misclassification of an unsafe state. The level set in black color is the single CBF's safe boundary. The ensemble avoids the collision by filtering the unreliable controls based on variance. Level sets in non-black colors represent the safe boundaries of other models from the ensemble. The high-variance region is shaded in pink. 
%\shnote{make figure text larger}
}
\label{fig::nav_ensemble}
\end{figure}

\section{Dynamics of Ego-Robots in Navigation Experiments} This section reports the dynamics used in our experiments.

% \todo[inline]{use standard symbols $x,y,v_x,v_y,u$ and equations.}

\subsubsection{Single Integrator}

The state $x=[p_x, p_y]$, where $p_x, p_y$ represent the Cartesian coordinates along the x and y axes. The action is the velocity along the x and y axes $u=[v_x, v_y]$, and the dynamics are given by $\dot p_x = v_x$, and $\dot p_y=v_y$. 

\subsubsection{Double Integrator}

The state $x=[p_x, p_y, v_x, v_y]$, representing Cartesian coordinates and velocities along the x and y axes. The action is the acceleration along the x and y axes $u=[a_x, a_y]$, and the dynamics are $\dot p_x = v_x$, $\dot p_{y} = v_y$, $\dot v_x = a_x$, and $\dot v_y=a_y$.
% \begin{equation}
% \dot x = \begin{bmatrix}
% 0 & 0 & 1 & 0 \\
% 0 & 0 & 0 & 1 \\
% 0 & 0 & 0 & 0 \\
% 0 & 0 & 0 & 0 
% \end{bmatrix}\cdot x + \begin{bmatrix}
% 0 & 0 \\
% 0 & 0 \\
% 1 & 0 \\
% 0 & 1 
% \end{bmatrix}\cdot u
% \end{equation}

\subsubsection{Dubins car}

The state $x=[p_x, p_y, v, \theta]$, where $p_x, p_y$ are the Cartesian coordinates, $v$ is the velocity on the xy plane, and $\theta$ is the heading angle of the car. The action is $u=[a, \omega]$, where $a$ is the acceleration and $\omega$ is the angular velocity. The dynamics are
$\dot p_x=v\cdot\cos(\theta)$, $\dot p_x=v \cdot \sin(\theta)$, $\dot v=a$, and $\dot \theta = \omega$.

% \begin{equation}
% \dot x =  \begin{bmatrix}
% v\cdot\cos(\theta) \\
% v \cdot \sin(\theta)\\
% 0\\
% 0
% \end{bmatrix} + \begin{bmatrix}
% 0 & 0 \\
% 0 & 0 \\
% 1 & 0 \\
% 0 & 1 
% \end{bmatrix}\cdot u
% \end{equation}

\subsubsection{Bicycle}

The state $x=[p_x, p_y, \theta, \delta]$, where $p_x, p_y$ are the Cartesian coordinates, $\theta$ is the heading angle, and $\delta$ is the steering angle. The action is $u=[v, \omega]$, where $v$ is the velocity, and $\omega$ is the angular velocity of $\delta$. Given the length of bicycle $L$, the dynamics are $\dot p_x=\frac{cos \theta}{L}v$, $\dot p_y = \frac{\sin \theta}{L}v$, $\dot \theta = \frac{\tan(\delta)}{L}v$, and $\dot \delta = \omega$.
%\begin{equation}
%\dot x = \begin{bmatrix}
%\frac{\cos(\theta)}{L} & 0 \\
%\frac{\sin(\theta)}{L} & 0 \\
%\frac{\tan(\delta)}{L} & 0 \\
%0 & 1 
%\end{bmatrix}\cdot u
%\end{equation}

\subsection{Detailed Results from Experiments}

% \todo[inline]{put the table here (i saw it commented out somewhere but can't find it now... i can find it in the history, let me know if you need that)}

We show the detailed performance in our experiments for navigation environment is shown in Table \ref{table::nav}.% (on next page). 

\begin{table*}[!bth]
\begin{adjustwidth}{-.85in}{-.85in}  
\centering\small
\begin{tabular}{|c|c|c|c|c|c|c|}
\hline
                       Dynamics            &      \diagbox{Method}{Obstacle Count}                  & 6           & 60          & 120         & 360         & 600         \\ \hline
\multirow{8}{*}{Dubins}            & NCBF                  & 0.00 (0.00) & 1.15 (0.10) & 3.47 (0.16) & 5.93 (0.27) & 10.9 (2.69) \\ \cline{2-7} 
                                   & NCBF (ensemble)       & 0.00 (0.00) & 0.00 (0.00) & 0.80 (0.09) & 1.31 (0.23) & 2.1 (1.02)  \\ 
                                     \cline{2-7}                                 & NCBF (non-sequential)   &  0.4 (0.09) & 6.77 (1.45) & 19.6 (3.58) &32.6 (3.24) & 49.3 (33.6)\\
                                   
                                   \cline{2-7} 
                                   & G-PFM                 & 0.90 (0.05) & 10.1 (1.0)  & 20.5 (0.48) & 55.4 (7.55) & 75.9 (5.09) \\ \cline{2-7} 
                                   & S-PFM                 & 0.00 (0.00) & 4.55 (0.14) & 10.1 (0.17) & 26.0 (3.83) & 40.7 (15.8) \\ \cline{2-7} 
                                   & B-MA-CBF              & 5.00 (0.67) & 12.8 (1.24) & 27.9 (2.41) & 95.0 (12.1) & 100. (0.00) \\ \cline{2-7} 
                                   & S-MPC                 & 0.00 (0.00) & 1.30 (0.16) & 2.14 (0.18) & 10.3 (0.79) & 20.5 (2.29) \\ \cline{2-7} 
                                   & S-MPC (true dynamics) & 0.00 (0.00) & 0.53 (0.08) & 1.05 (0.12) & 2.07 (0.39) & 7.50 (0.51) \\ \cline{2-7} 
                                   & PPO   &  16.00 (4.26) & 82.00 (0.81) & 94.17  (1.17) &100.00 (0.00) & 100.00 (0.00) \\
                                   
                                   \hline
\multirow{4}{*}{Single Integrator} & NCBF                  & 0.00 (0.00) & 1.09 (0.02) & 2.59 (0.02) & 3.94 (0.10) & 8.13 (0.47) \\ \cline{2-7} 
                                   & G-PFM                 & 0.00 (0.00) & 2.40 (0.13) & 6.77 (0.18) & 26.8 (1.94) & 53.7 (7.17) \\ \cline{2-7} 
                                   & S-PFM                 & 0.00 (0.00) & 0.30 (0.04) & 3.67 (0.15) & 9.35 (0.29) & 17.2 (1.10) \\ \cline{2-7} 
                                   & B-MA-CBF              & 3.33 (0.89) & 12.3 (0.53) & 25.9 (1.41) & 72.6 (10.5) & 99.3 (0.89) \\ \hline
\multirow{4}{*}{Double Integrator} & NCBF                  & 0.00 (0.00) & 0.69 (0.25) & 1.12 (0.63) & 9.70 (0.17) & 14.6 (0.20) \\ \cline{2-7} 
                                   & G-PFM                 & 1.27 (0.11) & 8.4 (0.33)  & 16.2 (0.82) & 61.0 (8.06) & 88.3 (11.6) \\ \cline{2-7} 
                                   & S-PFM                 & 0.00 (0.00) & 1.77 (0.07) & 3.13 (0.11) & 14.1 (2.43) & 36.9 (13.3) \\ \cline{2-7} 
                                   & B-MA-CBF              & 5.63 (1.47) & 17.3 (1.13) & 29.9 (2.77) & 99.3 (0.22) & 100. (0.00) \\ \hline
\multirow{4}{*}{Kinematic Bicycle} & NCBF                  & 0.00 (0.00) & 0.67 (0.22) & 5.57 (0.24) & 9.93 (0.40) & 16.2 (1.14) \\ \cline{2-7} 
                                   & G-PFM                 & 1.93 (0.51) & 13.0 (0.70) & 15.7 (3.15) & 54.1 (4.16) & 83.3 (14.0) \\ \cline{2-7} 
                                   & S-PFM                 & 0.00 (0.00) & 9.20 (0.32) & 16.0 (0.67) & 23.4 (1.42) & 37.3 (19.1) \\ \cline{2-7} 
                                   & B-MA-CBF              & 7.37 (0.95) & 21.0 (1.22) & 36.0 (2.67) & 100. (0.00) & 100. (0.00) \\ \hline
\end{tabular}
\end{adjustwidth}
\caption{ The overall collision rates (\%) in the navigation environment.}
\label{table::nav}
\end{table*}

%\subsection{Non-Sequential Models}

%In this section, we discuss the design choice of non-sequential CBF model. To ensure fair comparisons, we reveal more obstacle features (e.g. velocities and orientations) to the non-sequential neural CBF in our experiments. However it suffers from lacking generalizability, and delivers even worse performance than the potential-field controller's. The results are demonstrated in Table \ref{table::nav}. We attribute the cause to that spatial features provides only insufficient information. For instance, it's not plausible to estimate the interactions among obstacles based on merely obstacles' present information.
